# Supplementary material for: Statistical inference under response-adaptive experimental designs: a systematic review
Source: arXiv:2611.28380 source file (2026-11-20)
Supplement: Supplementary file 1 [file supplementary_methods-labels.tex]

% Generated from supplementary_methods.aux by scripts/build_documents.py.
% Label numbers/pages only: no external PDF hyperlinks or bibliography state.
\makeatletter
\@namedef{r@app:count-memberships}{{S2}{2}{}{}{}}
\@namedef{r@app:exclusions}{{S3}{15}{}{}{}}
\@namedef{r@app:prisma-abstract-checklist}{{S6}{24}{}{}{}}
\@namedef{r@app:prisma-checklist}{{S5}{19}{}{}{}}
\@namedef{r@app:search}{{S4}{18}{}{}{}}
\@namedef{r@app:topicmodel}{{S1}{1}{}{}{}}
\@namedef{r@tab:appexcl}{{S5}{15}{}{}{}}
\@namedef{r@tab:papersq1}{{S1}{2}{}{}{}}
\@namedef{r@tab:papersq2}{{S2}{6}{}{}{}}
\@namedef{r@tab:papersq3}{{S3}{8}{}{}{}}
\@namedef{r@tab:papersq4}{{S4}{11}{}{}{}}
\@namedef{r@tab:prismaabstractchecklist}{{S7}{24}{}{}{}}
\@namedef{r@tab:prismachecklist}{{S6}{19}{}{}{}}
\makeatother
